# Supplementary material for: Topological Data Analysis of Spatial Patterning in Heterogeneous Cell Populations: Clustering and Sorting with Varying Cell-Cell Adhesion
Source: arXiv:2212.14113 source file (2023-07-31)
Supplement: Supplementary file 1 [file 0_ABM.tex]

\subsection{Analytical Calculations for the ABM Model} 

In the absence of any random self-propulsion force, the equilibrium distance between particles, $r_{\text{eq}}$, is determined by the Morse potential parameters:

\begin{equation}
\label{eqn:ABM_Fexp}
    |\mathbf{F}_{ij}| = \gamma_{ij} \Bigg| \frac{1}{4l_R}\text{exp}\Big(-\frac{r_{ij}}{l_R}\Big)-\frac{1}{l_A}\text{exp}\Big(-\frac{r_{ij}}{l_A}\Big)\Bigg| = 0 \implies r_{\text{eq}}=\frac{l_Al_R}{l_A-l_R}\ln\Big(\frac{l_A}{4l_R}\Big) \approx 1.009
\end{equation}

The depth of the potential well is maximized at $r_{\text{eq}}$:

\begin{equation}
\label{eqn:ABM_Udepth}
    U(r_{\text{eq}}) = - \gamma_{ij} \Big( \frac{4l_R}{l_A}\Big)^\frac{l_R}{l_A-l_R} + \frac{\gamma_{ij}}{4} \Big( \frac{4l_R}{l_A}\Big)^\frac{l_A}{l_A-l_R} \approx -0.897 \gamma_{ij}
\end{equation}

\noindent The distance at which the force due to the Morse potential reaches local maximum lies outside the neighborhood distance $r_\text{max}$ (Eqn. \ref{eqn:ABM_dFdr}), therefore the maximum attraction and repulsion force occur at $r=r_\text{max}$ and $r=0$ respectively (Eqn. \ref{eqn:ABM_Fmax}):

\begin{equation}
\label{eqn:ABM_dFdr}
\frac{d|\mathbf{F}_{ij}|}{dr_{ij}} = 0 \implies r = \frac{l_Al_R}{l_A-l_R} \ln\Big(\frac{l_A^2}{4l_R^2}\Big) \approx 2.737 > r_{\text{max}}
\end{equation}

\begin{equation}
\label{eqn:ABM_Fmax}
    |\mathbf{F}_{ij}|_{\text{max}} = \begin{cases}
      \displaystyle
      \frac{l_A-4l_R}{4l_Al_R}\max(\gamma_{ij}) \approx 0.4286 \max(\gamma_{ij}), & \text{at}\ r_{ij}=0 \\
      \Big|\frac{1}{4l_R}\text{exp}\Big(-\frac{r_\text{max}}{l_R}\Big)-\frac{1}{l_A}\text{exp}\Big(-\frac{r_\text{max}}{l_A}\Big)\Big|\max(\gamma_{ij}) \approx 0.0393 \max(\gamma_{ij}), & \text{at}\ r_{ij}=r_\text{max}
      \end{cases}
\end{equation}

The ratio between the maximum attractive force and the polarization force varies between $0.078$ and $1.964$ for adhesion energy values $\gamma_{ij} \in [0.01, 0.25]$ and fixed polarization force magnitude, $|\mathbf{P}| = 0.005$. In a binary system, the polarization force dominates over the attractive adhesion force when $\gamma_{ij} < 0.127$. \textbf{TODO: account for random polarization}

\begin{equation}
\label{eqn:ABM_force_ratio}
0.078 < \frac{|\mathbf{F}_{ij}^{\text{attr}}|}{|\mathbf{P}_i|} = \frac{0.0393\gamma_{ij}}{0.005} < 1.964
\end{equation}
